# Supplementary material for: Scale Calibrated Training: Improving Generalization of Deep Networks via Scale-Specific Normalization
Source: arXiv:1909.00182 source file (2020-09-07)
Supplement: Supplementary file 1 [file appendix.tex]

\section{Appendix}

\begin{definition}[Lipschitz Continuity] A function $f$ is a Lipschitz continuous function on the set $\Omega$, if there exists a constant $K$ such that
\begin{equation}
    ||f(x_1) - f(x_2)|| \leq K ||x_1 - x_2||, \quad \forall x_1, x_2 \in \Omega.
\end{equation}
\end{definition}

\begin{example}[Counter-example] Consider the function 
\begin{align}
  f:  [0,1] & \rightarrow [0,1] \notag \\
  x & \mapsto \sqrt{x} \quad
\end{align}
$f$ is continuous on $[0,1]$, but $f$ is not Lipschitz continuous.    
\begin{proof}
If $f$ is Lipschitz continuous on $[0,1]$ with a Lipschitz constant $K>0$, then we have
\begin{equation*}
    ||\sqrt{x} - \sqrt{y}|| \leq K ||x-y||, \quad \forall x,y \in [0,1].
\end{equation*}
But taking a contradiction of $x=0$ and $y=\frac 1 {4K^2}$, we have
\begin{equation*}
    ||\sqrt{x} - \sqrt{y}|| = \frac 1 {2K} > \frac 1 {4K} = K||x-y||.
\end{equation*}
\end{proof}

\end{example}
